# Supplementary material for: End-to-End Spatio-Temporal Action Localisation with Video Transformers
Source: arXiv:2304.12160 source file (2023-04-24)
Supplement: Supplementary file 1 [file qualitative_examples.tex]

\section{Qualitative examples}
\label{sec:app_qualitative_examples}

Please refer to the attached supplementary video to see qualitative examples of our predicted tubelets on AVA and UCF101-24.
The video uses the ``H264 MP4'' codec, and has been tested on ``VLC Media Player'' and ``QuickTime''.
