# Supplementary material for: End-to-End Spatio-Temporal Action Localisation with Video Transformers
Source: arXiv:2304.12160 source file (2023-04-24)
Supplement: Supplementary file 2 [file supp_intro.tex]

In this supplementary material, we include qualitative examples (Sec.~\ref{sec:app_qualitative_examples}) and additional experiments and details (Sec.~\ref{sec:app_experiments}).
